# Supplementary material for: Online Normalization for Training Neural Networks
Source: arXiv:1905.05894 source file (2019-12-03)
Supplement: Supplementary file 1 [file appendix_streaming.tex]

\begin{itemize}
\item Math behind specific tensor-wide operations 
\item Forward pass statistics:  Exponential averaging, CoM, momentum 
\item Delta pass statistics: Control process, horizon
\end{itemize}
